# Supplementary material for: MeltNet: Predicting alloy melting temperature by machine learning
Source: arXiv:2010.14048 source file (2020-10-27)
Supplement: Supplementary file 1 [file SI.pdf]

Supporting Information For

# MeltNet: Predicting alloy melting temperature by machine learning

Pin-Wen Guan[1, a)] and Venkatasubramanian Viswanathan[1, 2, 3]

[1)]*Department of Mechanical Engineering, Carnegie Mellon University, Pittsburgh, Pennsylvania 15213, USA*

[2)]*Wilton E. Scott Institute for Energy Innovation, Carnegie Mellon University, Pittsburgh, Pennsylvania 15213, USA*

[3)]*Department of Physics, Carnegie Mellon University, Pittsburgh, Pennsylvania 15213, US*

(Dated: 27 October 2020)

[a)]Electronic mail: pinweng@andrew.cmu.edu

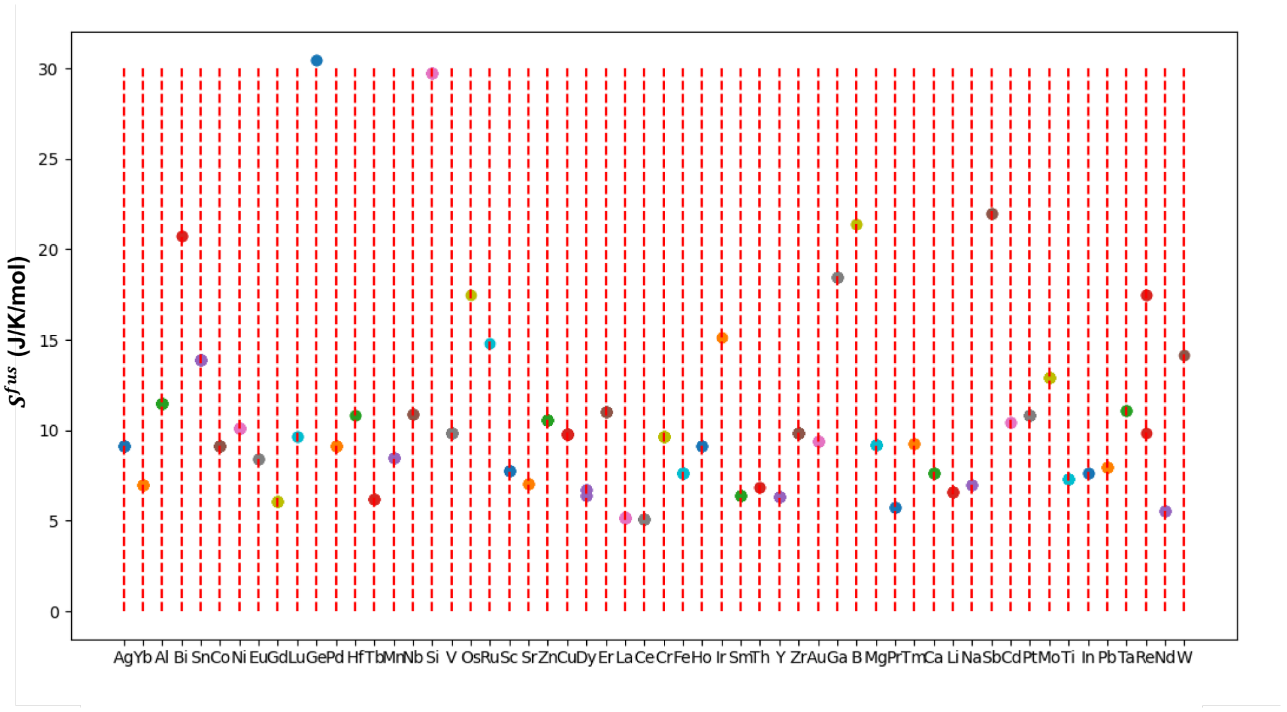


FIG. S1. Fusion entropy of elements involved in the present study.
